# Supplementary material for: A Modular Approach for Multilingual Timex Detection and Normalization using Deep Learning and Grammar-based methods
Source: arXiv:2304.14221 source file (2023-04-27)
Supplement: Supplementary file 1 [file appendix.tex]

% APPENDIX

% Gold Norm Results

\begin{table}[h!]
    \centering
    \begin{tabular}{l r r} \hline\hline
        System & TE3 Acc & MT Acc \\
        \hline\hline
        TimeNorm-en & \textbf{78.99} & \textbf{76.86} \\
        HeidelTime-en & 74.64 & 75.41 \\
        % HeidelTime-en & 72.46 & 75.62 \\ % Passing isolated timexes
        % UWTime AQ+TB-C & 82.61 & X \\
        % UWTime TB & 82.61 & X \\
        \hline
        TimeNorm-es & \textbf{80.40} & \textbf{72.57} \\
        HeidelTime-es & \textbf{80.40} & 71.61 \\
        % HeidelTime-es & 77.89 & 71.97 \\ % Passing isolated timexes
        \hline\hline
    \end{tabular}
    \caption{Results for normalization on isolated timexes from TempEval-3 and MEANTIME corpora.}
    \label{}
\end{table}

% Normalization of HeidelTime-detected timexes

\begin{table}[h!]
    \centering
    \begin{tabular}{l r r} \hline\hline
        System & TE3 VP & MT VP \\
        \hline\hline
        TimeNorm-en & 77.69 & 81.25 \\
        HeidelTime-en & \textbf{79.23} & \textbf{84.49} \\
        \hline
        TimeNorm-es & 83.52 & 72.34 \\
        HeidelTime-es & \textbf{90.91} & \textbf{72.98} \\
        \hline\hline
    \end{tabular}
    \caption{Normalization of HeidelTime-detected timexes (value precision).}
    \label{tab:results-norm-ht}
\end{table}

\begin{table}[h!]
    \centering
    \begin{tabular}{l r r} \hline\hline
        System & TE3 VAcc & MT VAcc \\
        \hline\hline
        TimeNorm-en & 83.47 & 85.37 \\
        HeidelTime-en & \textbf{85.12} & \textbf{89.02} \\
        \hline
        TimeNorm-es & 86.39 & 79.15 \\
        HeidelTime-es & \textbf{94.67} & \textbf{81.28} \\
        \hline\hline
    \end{tabular}
    \caption{Normalization of HeidelTime correctly detected timexes (value accuracy).}
    \label{tab:results-norm-ht}
\end{table}

\begin{table}[h!]
    \centering
    \begin{tabular}{l r r} \hline\hline
        System & TE3 VAcc & MT VAcc \\
        \hline\hline
        TimeNorm-en & \textbf{86.99} & 84.69 \\
        HeidelTime-en & 85.12 & \textbf{89.02} \\
        \hline
        TimeNorm-es & 84.44 & 77.08 \\
        HeidelTime-es & \textbf{94.67} & \textbf{81.28} \\
        \hline\hline
    \end{tabular}
    \caption{Normalization of correctly detected timexes by each system (value accuracy).}
    \label{tab:results-norm-ht}
\end{table}

% Det-Norm Results

% In Tables \ref{tab:results-det-norm-en-tb} and \ref{tab:results-det-norm-es-tb} we present the results for the TempEval-3 timex detection and evaluation tasks for English and Spanish, respectively. All the metrics refer to relaxed (``Rel") scores for precision (``P"), recall (``R") and/or F1 either for timex detection (``Rel P", ``Rel R" and ``Rel F1"), timex type (``Rel TF1") and timex value or normalization (``Rel VP", ``Rel VR" and ``Rel VF1"). System results at the top are those referred on the corresponding papers, whereas bottom results are the ones obtained according to our evaluation method. Similarly, Tables \ref{tab:results-det-norm-en-mt} and \ref{tab:results-det-norm-es-mt} show the results obtained by each system on English and Spanish MEANTIME.

% HeidelTime (GitHub): https://github.com/HeidelTime/heideltime/wiki/Evaluation-Results
% R2R*p: Best model in BERT got a date (Almasian et al., 2021) (Gertz included)
% UWTime: Lee et al., 2014 (Zettlemoyer included)
% Lange (BERT w/ AT): Lange et al., 2020 (Strötgen included)

% XLMR/Flair-TN-D: Cuentan las timexes detectadas no normalizadas (detection-focused).
% XLMR/Flair-TN-N: No cuentan las timexes detectadas no normalizadas (normalization-focused).
% UWTime AQ+TB-C: Trained on corrected AQUAINT and TimeBank.
% UWTime TB-C: Trained on corrected TimeBank.
% UWTime AQ+TB: Trained on original AQUAINT and TimeBank.
% UWTime SA: Results from UWTime Standalone.

\begin{table}[h!]
    \centering
    \begin{tabular}{l c c c c c c c}
        \hline\hline
        System & Rel P & Rel R & Rel F1 & Rel TF1 & Rel VP & Rel VR & Rel VF1 \\
        \hline\hline
        HeidelTime & 93.13 & 88.41 & 90.71 & 83.27 & X & X & 78.07 \\
        % HeidelTime TE3 & 93.08 & 87.68 & 90.30 & X & X & X & 77.61 \\
        % HeidelTime-13 & 93.08 & 87.68 & 90.30 & 82.09 & X & X & 77.61 \\
        % NewsReader & 84.71 & X & X & X & 72.16 \\
        % UWTime & \textbf{94.6} & \textbf{88.4} & \textbf{91.4} & \textbf{85.4} & \textbf{85.3} & \textbf{79.7} & \textbf{82.4} \\
        % SynTime-I & 94.29 & 95.65 & 94.96 & X & X & X & X \\
        % Lange & X & X & 86.61 & 79.53 & X & X & X \\
        % R2R*p & \textbf{100} & \textbf{100} & \textbf{100} & \textbf{90.43} & X & X & X \\
        \hline
        XTN-D & 93.53 & \textbf{94.20} & \textbf{93.86} & \textbf{88.81} & 76.98 & \textbf{77.54} & 77.26 \\
        XTN-N & \textbf{95.35} & 89.13 & 92.13 & 88.39 & 82.95 & \textbf{77.54} & 80.15 \\
        XTN-N Alt & (100) & (89.13) & (94.25) & (90.42) & \textbf{86.99} & \textbf{77.54} & \textbf{81.99} \\
        % Flair-TN-D & 93.89 & 89.13 & 91.45 & 84.76 & 77.10 & 73.19 & 75.09 \\
        % Flair-TN-N & \textbf{95.87} & 84.06 & 89.58 & 84.17 & 83.47 & 73.19 & 77.99 \\
        HeidelTime & 93.08 & 87.68 & 90.30 & 82.84 & 79.23 & 74.64 & 76.87 \\
        % UWTime AQ+TB-C & 94.53 & 87.68 & 90.98 & 85.71 & \textbf{85.94} & 79.71 & 82.71 \\
        % UWTime AQ+TB & 93.85 & 88.41 & 91.04 & 85.07 & 84.62 & 79.71 & 82.09 \\
        % UWTime TB-C & 91.97 & 91.30 & 91.64 & 85.82 & 82.48 & \textbf{81.88} & 82.18 \\
        % UWTime TB & 93.85 & 88.41 & 91.04 & 87.31 & 85.38 & 80.43 & \textbf{82.84} \\
        % UWTime SA & 91.97 & 91.30 & 91.64 & 85.82 & 82.48 & \textbf{81.88} & 82.18 \\
        \hline\hline
    \end{tabular}
    \caption{Results for English TempEval-3 timex detection and normalization task.}
    \label{tab:results-det-norm-en-tb}
\end{table}

\begin{table}[h!]
    \centering
    \begin{tabular}{l c c c c c c c}
        \hline\hline
        System & Rel P & Rel R & Rel F1 & Rel TF1 & Rel VP & Rel VR & Rel VF1 \\
        \hline\hline
        HeidelTime & 96.02 & 84.92 & 90.13 & 87.47 & X & X & \textbf{85.33} \\
        % HeidelTime TE3 & 96.0 & 84.9 & 90.1 & X & X & X & \textbf{87.5} \\
        % HeidelTime-13 & 96.02 & 84.92 & 90.13 & 87.47 & X & X & 85.33 \\
        % NewsReader & X & X & X & 85.33 \\
        % Lange & X & X & 85.71 & 80.11 & X & X & X \\
        \hline
        XTN-D & 97.47 & \textbf{96.98} & \textbf{97.23} & \textbf{93.20} & 76.77 & 76.38 & 76.57 \\
        XTN-N & \textbf{98.36} & 90.45 & 94.24 & 91.10 & 83.06 & 76.38 & 79.58 \\
        XTN-N Alt & (100) & (90.45) & (94.99) & (91.82) & 84.44 & 76.38 & 80.21 \\
        % Flair-TN-D & 96.88 & 93.47 & 95.14 & 91.56 & 78.65 & 75.88 & 77.24 \\
        % Flair-TN-N & 96.76 & 89.95 & 93.23 & 90.10 & 81.62 & 75.88 & 78.65 \\
        HeidelTime & 96.02 & 84.92 & 90.13 & 87.47 & \textbf{90.91} & \textbf{80.40} & \textbf{85.33} \\
        \hline\hline
    \end{tabular}
    \caption{Results for Spanish TempEval-3 timex detection and normalization task.}
    \label{tab:results-det-norm-es-tb}
\end{table}

\begin{table}[h!]
    \centering
    \begin{tabular}{l c c c c c c c}
        \hline\hline
        System & Rel P & Rel R & Rel F1 & Rel TF1 & Rel VP & Rel VR & Rel VF1 \\
        \hline\hline
        % NewsReader & 80.50 & X & X & X & 68.50 \\
        % \hline
        XTN-D & 94.33 & \textbf{92.77} & \textbf{93.54} & \textbf{88.33} & 76.47 & 75.21 & 75.83 \\
        XTN-N & \textbf{95.99} & 89.05 & 92.39 & 87.46 & 81.29 & \textbf{75.41} & 78.24 \\
        XTN-N Alt & (98.85) & (89.05) & (93.70) & (88.70) & 83.72 & \textbf{75.41} & 79.35 \\
        % Flair-TN-D & \textbf{98.33} & 85.12 & 91.25 & 85.71 & 82.58 & 71.49 & 76.63 \\
        % Flair-TN-N & 98.26 & 81.61 & 89.16 & 84.65 & \textbf{86.07} & 71.49 & 78.10 \\
        HeidelTime & 94.91 & 84.71 & 89.52 & 85.15 & \textbf{84.49} & \textbf{75.41} & \textbf{79.69} \\
        % UWTime SA & 87.14 & 86.78 & 86.96 & 82.82 & 65.56 & 65.29 & 65.42 \\
        \hline\hline
    \end{tabular}
    \caption{Results for timex detection and normalization on English MEANTIME.}
    \label{tab:results-det-norm-en-mt}
\end{table}

\begin{table}[h!]
    \centering
    \begin{tabular}{l c c c c c c c}
        \hline\hline
        System & Rel P & Rel R & Rel F1 & Rel TF1 & Rel VP & Rel VR & Rel VF1 \\
        \hline\hline
        % NewsReader & 78.30 & X & X & X & 62.20 \\
        % \hline
        XTN-D & 91.43 & \textbf{95.82} & \textbf{93.58} & \textbf{86.03} & 68.13 & 71.40 & 69.72 \\
        XTN-N & \textbf{92.32} & 92.90 & 92.61 & 85.33 & 71.16 & \textbf{71.61} & 71.38 \\
        XTN-N Alt & (98.89) & (92.90) & (95.80) & (88.27) & \textbf{76.22} & \textbf{71.61} & \textbf{73.84} \\
        % Flair-TN-D & 91.22 & 93.32 & 92.26 & 85.86 & 68.98 & 70.56 & 69.76 \\
        % Flair-TN-N & 92.02 & 91.44 & 91.73 & 85.65 & 71.01 & 70.56 & 70.79 \\
        HeidelTime & 89.79 & 88.10 & 88.94 & 81.35 & 72.98 & \textbf{71.61} & 72.29 \\
        \hline\hline
    \end{tabular}
    \caption{Results for timex detection and normalization on Spanish MEANTIME.}
    \label{tab:results-det-norm-es-mt}
\end{table}

% Comparison with UWTime

\begin{table}[h!]
    \centering
    \begin{tabular}{l c c c c c c c}
        \hline\hline
        System & Rel P & Rel R & Rel F1 & Rel TF1 & Rel VP & Rel VR & Rel VF1 \\
        \hline\hline
        XTN-D TB & 93.53 & 94.20 & 93.86 & 88.81 & 76.98 & 77.54 & 77.26 \\
        XTN-N TB & 95.35 & 89.13 & 92.13 & 88.39 & 82.95 & 77.54 & 80.15 \\
        XTN-D TB-C & 93.66 & \textbf{96.38} & \textbf{95.00} & \textbf{90.71} & 75.35 & 77.54 & 76.43 \\
        XTN-N TB-C & \textbf{95.42} & 90.58 & 92.94 & 89.96 & 81.68 & 77.54 & 79.55 \\
        XTN-D TBAQ & 94.03 & 91.30 & 92.65 & 86.03 & 76.87 & 74.64 & 75.74 \\
        XTN-N TBAQ & 95.24 & 86.96 & 90.91 & 85.61 & 82.54 & 75.36 & 78.79 \\
        XTN-D TBAQ-C & 94.07 & 92.03 & 93.04 & 89.38 & 80.00 & 78.26 & 79.12 \\
        XTN-N TBAQ-C & 95.35 & 89.13 & 92.13 & 89.14 & 83.72 & 78.26 & 80.90 \\
        \hline
        UWTime TB & 93.85 & 88.41 & 91.04 & 87.31 & 85.38 & 80.43 & \textbf{82.84} \\
        UWTime TB-C & 91.97 & 91.30 & 91.64 & 85.82 & 82.48 & \textbf{81.88} & 82.18 \\
        UWTime TBAQ & 93.85 & 88.41 & 91.04 & 85.07 & 84.62 & 79.71 & 82.09 \\
        UWTime TBAQ-C & 94.53 & 87.68 & 90.98 & 85.71 & \textbf{85.94} & 79.71 & 82.71 \\
        UWTime SA & 91.97 & 91.30 & 91.64 & 85.82 & 82.48 & \textbf{81.88} & 82.18 \\
        \hline
        HeidelTime & 93.08 & 87.68 & 90.30 & 82.84 & 79.23 & 74.64 & 76.87 \\
        \hline\hline
    \end{tabular}
    \caption{English TE3 results given original and UWTime-corrected corpora.}
    \label{tab:results-det-norm-en-tb}
\end{table}

\begin{table}[h!]
    \centering
    \begin{tabular}{l c c c c c c c}
        \hline\hline
        System & Rel P & Rel R & Rel F1 & Rel TF1 & Rel VP & Rel VR & Rel VF1 \\
        \hline\hline
        XTN-D TB & 97.47 & \textbf{96.98} & \textbf{97.23} & \textbf{93.20} & 76.77 & 76.38 & 76.57 \\
        XTN-N TB & 98.36 & 90.45 & 94.24 & 91.10 & 83.06 & 76.38 & 79.58 \\
        XTN-D TB-C & 95.45 & 94.97 & 95.21 & 90.68 & 75.76 & 75.38 & 75.57 \\
        XTN-N TB-C & 97.27 & 89.45 & 93.19 & 89.01 & 81.97 & 75.38 & 78.53 \\
        XTN-D TBAQ & 97.44 & 95.48 & 96.45 & 91.37 & 77.44 & 75.88 & 76.65 \\
        XTN-N TBAQ & \textbf{98.90} & 90.45 & 94.49 & 90.29 & 82.97 & 75.88 & 79.27 \\
        XTN-D TBAQ-C & 94.97 & 94.97 & 94.97 & 91.96 & 74.87 & 74.87 & 74.87 \\
        XTN-N TBAQ-C & 97.24 & 88.44 & 92.63 & 89.47 & 82.32 & 74.87 & 78.42 \\
        \hline
        HeidelTime & 96.02 & 84.92 & 90.13 & 87.47 & \textbf{90.91} & \textbf{80.40} & \textbf{85.33} \\
        \hline\hline
    \end{tabular}
    \caption{Spanish TE3 results given original and UWTime-corrected corpora.}
    \label{tab:results-det-norm-es-tb}
\end{table}

\begin{table}[h!]
    \centering
    \begin{tabular}{l c c c c c c c}
        \hline\hline
        System & Rel P & Rel R & Rel F1 & Rel TF1 & Rel VP & Rel VR & Rel VF1 \\
        \hline\hline
         XTN-D TB & 94.33 & \textbf{92.77} & \textbf{93.54} & \textbf{88.33} & 76.47 & 75.21 & 75.83 \\
        XTN-N TB & 95.99 & 89.05 & 92.39 & 87.46 & 81.29 & \textbf{75.41} & 78.24 \\
        \hline
        XTN-D TB-C & 94.81 & 94.42 & 94.62 & 88.61 & 76.97 & 76.65 & 76.81 \\
        XTN-N TB-C & 96.08 & 91.12 & 93.53 & 87.80 & 80.83 & 76.65 & 78.69 \\
        XTN-D TBAQ & 94.32 & 89.26 & 91.72 & 86.84 & 77.73 & 73.55 & 75.58 \\
        XTN-N TBAQ & 95.67 & 86.78 & 91.01 & 86.24 & 81.09 & 73.55 & 77.14 \\
        XTN-D TBAQ-C & 94.93 & 92.77 & 93.83 & 86.73 & 77.38 & 75.62 & 76.49 \\
        XTN-N TBAQ-C & 95.36 & 89.26 & 92.21 & 85.38 & 80.79 & 75.62 & 78.12 \\
        \hline
        Flair-TN-D & \textbf{98.33} & 85.12 & 91.25 & 85.71 & 82.58 & 71.49 & 76.63 \\
        Flair-TN-N & 98.26 & 81.61 & 89.16 & 84.65 & \textbf{86.07} & 71.49 & 78.10 \\
        HeidelTime & 94.91 & 84.71 & 89.52 & 85.15 & 84.49 & \textbf{75.41} & \textbf{79.69} \\
        UWTime SA & 87.14 & 86.78 & 86.96 & 82.82 & 65.56 & 65.29 & 65.42 \\
        \hline\hline
    \end{tabular}
    \caption{English MEANTIME results given original and UWTime-corrected corpora.}
    \label{tab:results-det-norm-es-tb}
\end{table}

\begin{table}[h!]
    \centering
    \begin{tabular}{l c c c c c c c}
        \hline\hline
        System & Rel P & Rel R & Rel F1 & Rel TF1 & Rel VP & Rel VR & Rel VF1 \\
        \hline\hline
        XTN-D TB & 91.43 & \textbf{95.82} & \textbf{93.58} & \textbf{86.03} & 68.13 & 71.40 & 69.72 \\
        XTN-N TB & \textbf{92.32} & 92.90 & 92.61 & 85.33 & 71.16 & \textbf{71.61} & 71.38 \\
        \hline
        XTN-D TBAQ & 89.84 & 96.03 & 92.84 & 85.17 & 66.41 & 70.98 & 68.62 \\
        XTN-N TBAQ & 91.89 & 94.57 & 93.21 & 85.60 & 69.17 & 71.19 & 70.16 \\
        \hline
        Flair-TN-D & 91.22 & 93.32 & 92.26 & 85.86 & 68.98 & 70.56 & 69.76 \\
        Flair-TN-N & 92.02 & 91.44 & 91.73 & 85.65 & 71.01 & 70.56 & 70.79 \\
        HeidelTime & 89.79 & 88.10 & 88.94 & 81.35 & \textbf{72.98} & \textbf{71.61} & \textbf{72.29} \\
        \hline\hline
    \end{tabular}
    \caption{Spanish MEANTIME results given original and UWTime-corrected corpora.}
    \label{tab:results-det-norm-es-tb}
\end{table}
